# Supplementary material for: On the Relationship of Optimal State Feedback and Disturbance Response Controllers
Source: arXiv:2304.03831 source file (2023-04-07)
Supplement: Supplementary file 1 [file Appendix-optimal-disturbance.tex]

\section{Proof of Lemma \ref{lemma:optimal-L-K}}\label{apdx:optimal-LK}
We further define some variables that will be used in this section. Define the matrices $\Lambda_{km}\in \bR^{n_x\times n_x}$ as:
\begin{align}\label{eq:def-Lambda}
   \Lambda_{km}&:= \begin{cases}
         GA^{k-m}, &  k\ge m\\
         (A^{m-k})^\top G, & k<m 
    \end{cases} , \quad k,m\ge 1.
\end{align}
Define  ${\bf{A}}^{(H)} \in \mathbb{R}^{n_x\times H n_x}$ as:
\begin{align*}
    {\bf{A}}_k^{(H)} &:= 
    \begin{cases}
        [A^{k-1}, A^{k-2},\dots, A, I, 0,\dots, 0], & k< H \\
        \left[A^{k-1},A^{k-2},\dots,A^{k-K}\right], & k\ge H
    \end{cases}
\end{align*}
Then, define $\mathbf\Lambda^{(H)} \!\in\! \bR^{Hn_x\times Hn_x }, \XiK\!\in\! \bR^{Hn_x\times Hn_x }, \BK\in\bR^{Hn_x \times Hn_u},\RK\in\bR^{Hn_u\times Hn_u},\SK\in\bR^{Hn_u\times Hn_x}$ as
\begin{align}
   \mathbf\Lambda^{(H)} &\!:=
    \begin{bmatrix}
         \Lambda_{11}& \Lambda_{12}&\cdots &\Lambda_{1H} \\
         \Lambda_{21}& \Lambda_{22}&\cdots &\Lambda_{2H}\\
         \vdots&\vdots & &\\
         \Lambda_{H1} & \Lambda_{H2}&\cdots &\Lambda_{HH}
    \end{bmatrix},~~
    \XiK\!:= \begin{bmatrix}
     0\\
     \mathbf A_1^{(H)}\\
     \vdots\\
     \mathbf A_{H-1}^{(H)}
    \end{bmatrix}\label{eq:def-Lambda-K},\\
    \BK&:= 
    \begin{bmatrix}
         B& &\\
          & \ddots&\\
          & &B
    \end{bmatrix},\quad 
    \RK:= \begin{bmatrix}
         R& &\\
          & \ddots&\\
          & &R
    \end{bmatrix},\vspace{3pt}\\
    &\qquad\qquad \qquad  \SK:= \begin{bmatrix}
         S& &\\
          & \ddots&\\
          & &S
    \end{bmatrix}. \label{eq:def-BK-RK}
\end{align}

We first prove the following lemma which writes out $C(\LK)$ explicitly.
\begin{lem}
The cost function defined in \eqref{eq:LQR-disturbanc-feedback} satisfies
\begin{equation*}
\begin{split}
    C(\LK) &\!=\! \tr\!\left(\!
    [I, \LK{}^\top]\!\left(\!
    \begin{bmatrix}
        I & 0 \\
        0 & \BK
    \end{bmatrix}^{\!\top}
    \!\!\!\LambdaK\!
    \begin{bmatrix}
        I & 0 \\
        0 & \BK
    \end{bmatrix}
    \right.\right.\\
    &+ \begin{bmatrix}
        0 & 0 \\
        0 & \RK
    \end{bmatrix}
    + 
    \begin{bmatrix}
        0 & 0 \\
        0 & \SK
    \end{bmatrix}
    \mathbf{\Xi}^{(H+1)}
    \begin{bmatrix}
        I & 0 \\
        0 & {\BK}
    \end{bmatrix}\\
   & +     \begin{bmatrix}
        I & 0 \\
        0 & {\BK}^\top
    \end{bmatrix}
    \mathbf{\Xi}^{(H+1)^\top}
\begin{bmatrix}
        0 & 0 \\
        0 & {\SK}^\top
    \end{bmatrix}
    \bigg)
    \begin{bmatrix}
         I  \\
         \LK 
    \end{bmatrix}
    \bigg).
\end{split}
\end{equation*}
\end{lem}
\begin{pf}
%\lina{if we use the complex domain to do the proof, we should make the proof more rigorous by defining things in a more mathematical rigorous way. but also a question is that do we need to go with the ``transform" and transfer function to do the proof? I feel is more straightfoward to just use the state-space solution to show the results. It is straightforward algebra.}

We denote the $z$-transform of $\{x_t\}, \{u_t\}, \{w_t\}$ as %\lina{technically, ``transfer function'' referring to the system transfer function. It is kind of ``Z-transform" but ``z=1/s'' in the definition. need to change transfer function to be a more accurate term. Also in order to make things more accurate, needs to specify $w_t$ for $t=-K:-1$}
\begin{align*}
    X(z):=\sum_{t=0}^\infty z^{-t} x_t,~~ U(z):=\sum_{t=0}^\infty z^{-t} u_t, ~~W(z):=\sum_{t=0}^\infty z^{-t} w_t.
\end{align*}
Let $$\LK(z):= z^{-1}\LK_1 + z^{-2}\LK_2 +\dots + z^{-H}\LK_H.$$
Then we have 
\begin{align*}
    \begin{cases}
    U(z) = \LK(z)W(z)\\
    X(z) = z^{-1}\left(AX(z)+BU(z)+W(z)\right) 
    \end{cases}\\
    \Rightarrow\quad 
    (I-z^{-1}A)X(z) = z^{-1}(I+B\LK(z))W(z),
\end{align*}
which gives
\begin{align*}
    % U(z) &= \LK(z)W(z),\\
    % X(z) &= z^{-1}AX(z) + z^{-1}BU(z) + z^{-1}W(z)\\
    % &= z^{-1}AX(z) + z^{-1}(I+B\LK(z))W(z)\\
    % \Longrightarrow~~ 
    &\quad X(z)= z^{-1}(I-z^{-1}A)^{-1}(I+B\LK(z))W(z)\\
    &= z^{-1}(I+z^{-1}A+z^{-2}A^2 +\dots)\\
    &\qquad(I+z^{-1}B\LK_1+z^{-2}B\LK_2 +\dots z^{-H}B\LK_H)W(z)\\
    & = \left(z^{-1}I + z^{-2} (A + B\LK_1)\right. \\
    &\qquad \left.+ z^{-3} (A^2 + AB\LK_1 + B\LK_2) + \cdots\right)W(z)\\
    &= \left(z^{-1}T_1 + z^{-2}T_2 + \cdots+ z^{-k} T_k + \cdots\right)W(z),
\end{align*}
where (we can derive by algebraic calculation)
\begin{align*}
    T_k = \AK 
    \begin{bmatrix}
        I & 0 \\
        0 & \BK
    \end{bmatrix}
    \begin{bmatrix}
         I  \\
         \LK 
    \end{bmatrix}.
\end{align*}
Thus we have that
\begin{align*}
    &\quad \lim_{T\to+\infty} \frac{1}{T}\mathbb{E}\sum_{t=0}^{T-1}x_t^\top Qx_t = \lim_{T\to+\infty}\frac{1}{T}\mathbb{E}\sum_{t=0}^{T-1}\tr(x_tx_t^\top Q) \\
    & = \tr\left(\sum_{t=1}^{+\infty} T_tT_t^\top Q\right)\quad \textup{(Lemma \ref{lemma:tf-second-moment})}\\
    & = \tr\left(\sum_{t=1}^{+\infty} T_t^\top QT_t\right) \\
    &= \tr\left([I,\LK{}^\top]
    \begin{bmatrix}
        I & 0 \\
        0 & \BK
    \end{bmatrix}^\top\left(\sum_{t=1}^{+\infty}\mathbf{A}_t^{(H+1)}{}^\top Q\mathbf{A}_t^{(H+1)}\right)\right.\\
    &\qquad\qquad\qquad\qquad\qquad\qquad\qquad\quad\left.\quad 
    \begin{bmatrix}
        I & 0 \\
        0 & \BK
    \end{bmatrix}
    \begin{bmatrix}
         I  \\
         \LK 
    \end{bmatrix}\right)\\
    &= \tr\left(\![I,\LK{}^\top\!]\!
    \begin{bmatrix}
        I & \!\!0 \\
        0 & \!\!\BK
    \end{bmatrix}^\top\!\!\!\!\!\!\LambdaK\!
    \begin{bmatrix}
        I & 0 \\
        0 & \BK
    \end{bmatrix}\!\!
    \begin{bmatrix}
         I  \\
         \LK 
    \end{bmatrix}\!\right),
\end{align*}
where the last equation follows from Lemma \ref{lemma:matrix-M} in Appendix \ref{apdx:auxiliary}. Similarly
\begin{align*}
    &\quad \lim_{T\to+\infty} \frac{1}{T}\mathbb{E}\sum_{t=0}^{T-1}u_t^\top Sx_t = \lim_{T\to+\infty}\frac{1}{T}\mathbb{E}\sum_{t=0}^{T-1}\tr(x_tu_t^\top S) \\
    & = \tr\left(\sum_{t=1}^{K} T_t{\LK_t}^\top S\right)\quad \textup{(Lemma \ref{lemma:tf-second-moment})}\\
    & = \tr\left(\sum_{t=1}^{K} {\LK_t}^\top ST_t\right) \\
    &= \tr\left(\LK{}^\top \SK \begin{bmatrix}
         T_1\\
         \vdots\\
         T_K
    \end{bmatrix}\right) \\
    &= \tr\left(
    \LK{}^\top\SK
    \begin{bmatrix}
         \mathbf{A}_1^{(H+1)}\\
         \vdots\\
         \mathbf{A}_K^{(H+1)}
    \end{bmatrix}
    \begin{bmatrix}
        I & 0 \\
        0 & \BK
    \end{bmatrix}
    \begin{bmatrix}
         I  \\
         \LK 
    \end{bmatrix}\right)\\
    &= \tr\!\left(\![I,\LK{}^\top]\!
     \begin{bmatrix}
        0 & 0 \\
        0 & \SK
    \end{bmatrix}
    \mathbf{\Xi}^{(H+1)}\!
    \begin{bmatrix}
        I & 0 \\
        0 & {\BK}
    \end{bmatrix}\!
    \begin{bmatrix}
         I  \\
         \LK 
    \end{bmatrix}\!\right)
\end{align*}

Additionally
\begin{align*}
    &\quad \lim_{T\to+\infty} \frac{1}{T}\mathbb{E}\sum_{t=0}^{T-1}u_t^\top Ru_t = \lim_{T\to+\infty} \frac{1}{T}\mathbb{E}\sum_{t=0}^{T-1}\tr(u_tu_t^\top R) \\
    &= \tr\left(\sum_{t=1}^{K} \LK_t\LK_t{}^\top R\right)\quad \textup{(Lemma \ref{lemma:tf-second-moment})}\\
    & = \tr\left(\sum_{t=1}^{K} \LK_t{}^\top R\LK_t\right) = \tr\left(\LK{}^\top \RK~\LK\right).
\end{align*}
Combining the two equations together we have that
\begin{equation*}
\begin{split}
    C(\LK&) \!=\! \tr\!\left(\!
    [I, \!\LK{}^\top]\!\left(\!
    \begin{bmatrix}
        I & 0 \\
        0 & \BK
    \end{bmatrix}^\top
    \!\!\!\!\!\LambdaK\!
    \begin{bmatrix}
        I & 0 \\
        0 & \BK
    \end{bmatrix}\right.\right.\\
    &
    + \begin{bmatrix}
        0 & 0 \\
        0 & \RK
    \end{bmatrix}
    + 
    \begin{bmatrix}
        0 & 0 \\
        0 & \SK
    \end{bmatrix}
    \mathbf{\Xi}^{(H+1)}
    \begin{bmatrix}
        I & 0 \\
        0 & {\BK}
    \end{bmatrix}\\
    &\left.\left.+     \begin{bmatrix}
        I & 0 \\
        0 & {\BK}^\top
    \end{bmatrix}
    \mathbf{\Xi}^{(H+1)^\top}
\begin{bmatrix}
        0 & 0 \\
        0 & {\SK}^\top
    \end{bmatrix}
    \right)
    \begin{bmatrix}
         I  \\
         \LK 
    \end{bmatrix}
    \right).
\end{split}
\end{equation*}
\end{pf}

Lemma \ref{lemma:optimal-L-K} is a direct corollary of the above lemma.
\begin{pf}(of Lemma \ref{lemma:optimal-L-K})

\begin{align*}
    C(\LK&) \!=\! \tr\!\left(\!
    [I, \!\LK{}^\top]\!\left(\!
    \begin{bmatrix}
        I & 0 \\
        0 & \BK
    \end{bmatrix}^\top
    \!\!\!\!\!\LambdaK\!
    \begin{bmatrix}
        I & 0 \\
        0 & \BK
    \end{bmatrix}\right.\right.\\
    &
    + \begin{bmatrix}
        0 & 0 \\
        0 & \RK
    \end{bmatrix}
    + 
    \begin{bmatrix}
        0 & 0 \\
        0 & \SK
    \end{bmatrix}
    \mathbf{\Xi}^{(H+1)}
    \begin{bmatrix}
        I & 0 \\
        0 & {\BK}
    \end{bmatrix}\\
    &\left.\left.+     \begin{bmatrix}
        I & 0 \\
        0 & {\BK}^\top
    \end{bmatrix}
    \mathbf{\Xi}^{(H+1)^\top}
\begin{bmatrix}
        0 & 0 \\
        0 & {\SK}^\top
    \end{bmatrix}
    \right)
    \begin{bmatrix}
         I  \\
         \LK 
    \end{bmatrix}
    \right).\\
    &=\tr\left(
    [I, \LK{}^\top]
    \begin{bmatrix}
        \Lambda_{11} & \HK{}^\top \\
        \HK & \MK
    \end{bmatrix}
    \begin{bmatrix}
         I  \\
         \LK 
    \end{bmatrix}
    \right),
\end{align*}
where the last equation can be verified by the definition of $\LambdaK,\XiK,\MK,\HK$. The last equation immediately leads to the fact that the optimal $\LK$ should solve
\begin{equation*}
\MK\LK + \HK=0.
\end{equation*}
\end{pf}
